# Supplementary material for: Algorithms for Fair Team Formation in Online Labour Marketplaces
Source: arXiv:2002.11621 source file (2020-02-14)
Supplement: Supplementary file 1 [file appendix.tex]

\section{Proof of Lemma 1}

\begin{proof}
The proof has similarities to the one used for proving the
approximation ratio for the set-cover
problem~\cite{vazirani2013approximation}, which we adapt to our
setting.

Consider the skills $\worker{r}\cap\atask$ sorted in the order that are
covered by \greedy, breaking ties arbitrarily. That is,
if $\Card{\worker{r}\cap\atask}=q$, if 
$\skill{i_1}, \skill{i_2}, \dots,\skill{i_q}$ are the skills in
$\worker{r}\cap\atask$, and if, say,
$\skill{i_1}, \dots, \skill{i_4}$ were covered by the most cost-efficent
worker, $\skill{i_5},\dots, \skill{i_{10}}$ by the second most
cost-efficient worker, and so on, until skllls
$\skill{i_s},\dots,\skill{i_q}$ covered by worker $\worker{r}$, then the
order that we consider for these skills is $\skill{i_1}, \skill{i_2},
\dots,\skill{i_q}$.

Consider the iteration of the \greedy algorithm that a
given element
$\skill{i_j}$ was covered. At that moment there are at least $q-j+1$
skills in $\worker{r}\cap\atask$ that have not been covered. Therefore, the cost efficiency of
worker $\worker{r}$ is at most $\outsourcecost{r}/(q-j+1)$. Because the
greedy algorithm covers each skill with the most cost-efficient worker, skill
$\skill{i_j}$ was covered by a worker $\worker{r'}$ (possibly $r'=r$) with cost
efficiency at most $\outsourcecost{r}/(q-j+1)$. Skills
are covered by workers with at least as high cost efficiency as
$\worker{r}$, until all the skills in $\worker{r}\cap\atask$ have been
covered; note that eventually all these skill are covered, the last
such skills being covered either by worker \worker{r} or by a more
cost-efficient worker.
Therefore, recalling that the price assigned to a skill is the cost efficiency
of the worker at the time that the skill was covered, for all $j=1\dots,q$ we have that
\[\price{\skill{i_j}}\le\frac{\outsourcecost{r}}{q-j+1}.\]
Hence,
%TOFIX
\[
\begin{split}
\sum_{\askill\in\worker{r}\cap\atask}\price{\askill}&=\sum_{j=1}^q\price{\skill{i_j}}
\le\sum_{j=1}^q\frac{\outsourcecost{r}}{q-j+1}\\
&=\outsourcecost{r}\cdot H_q\le \outsourcecost{r}\cdot H_\numskills.
\end{split}
\]
%Consider the elements in $\worker{r}$ sorted in the order they are covered by the greedy algorithm,
%and assume that $|\worker{r}|=k$. Let $\ell_1,\ell_2,\ldots ,\ell_k$ be that order.
%At the iteration when $\ell_i$ is covered, $\worker{r}$ contains $k-i+1$ uncovered elements. At 
%that iteration the cost-efficiency of $\worker{r}$ is $\frac{\outsourcecost{r}}{k-i+1}$.
%So, $\text{price}(\ell_i)\leq \frac{\outsourcecost{r}}{k-i+1}$ and therefore,
%
%\begin{eqnarray*}
%\sum_{\ell\in \task{t} \cap \worker{r}} \text{price}(\ell)& \leq & \outsourcecost{r}H_k\\
%& \leq &  \outsourcecost{r}H_m .
%\end{eqnarray*}
\end{proof}
